# Supplementary material for: cViL: Cross-Lingual Training of Vision-Language Models using Knowledge Distillation
Source: arXiv:2206.03354 source file (2022-06-09)
Supplement: Supplementary file 1 [file table_hin_supplementary.tex]

% \begin{table}[!h]
% \begin{center}
\begin{threeparttable}
\begin{tabular}{lc}
\toprule
\textbf{Model} & \textbf{Accuracy} \\
\midrule
% BUTD\textsuperscript{*}~\citep{gupta-etal-2020-unified} & $60.15$ \\
% Bi-linear Attention\textsuperscript{*}~\citep{gupta-etal-2020-unified} & $62.50$ \\
% Gupta \etal{}\textsuperscript{*}\citep{gupta-etal-2020-unified} & $64.51$ \\
% \midrule
% \modelbase & $68.14$ \\
% \modeltwo & $\textbf{71.74}$ \\
\modelbase & $67.09$ \\
\modeltwo & $\textbf{72.04}$ \\
\modelthree & $\textbf{72.04}$ \\
\bottomrule
\end{tabular}
% \begin{tablenotes}
% \item [*] They use the translated version of VQA 1.0, instead of VQA 2.0.
% \item [] 
% \end{tablenotes}
\end{threeparttable}
% \end{center}
% \caption{Evaluation results on the Hindi version of VQA 2.0 dataset.}
% \label{tab:hin_results}

% \end{table}
