# Supplementary material for: cViL: Cross-Lingual Training of Vision-Language Models using Knowledge Distillation
Source: arXiv:2206.03354 source file (2022-06-09)
Supplement: Supplementary file 2 [file table_jap_supplementary.tex]

% \begin{table}[!h]
% \begin{center}
\begin{threeparttable}
\begin{tabular}{lcc}
\toprule
\textbf{Model} & \textbf{Accuracy} & \textbf{BLEU} \\
\midrule
% PCATT\textsuperscript{*}~\citep{shimizu-etal-2018-visual} & $19.2$ & - \\
% UNITER\textsubscript{CC}~\citep{ChenLYK0G0020,zhou2021uc} & $22.7$ & $11.8$ \\
% UC\textsuperscript{2}~\citep{zhou2021uc} & $34.2$ & $26.8$ \\
% \midrule
\modelbase & $33.75$ & $28.1$ \\
\modelone & $34.93$ & $29.5$ \\
\modeltwo & $\textbf{35.72}$ & $\textbf{29.5}$ \\
\modelthree & $\textbf{35.72}$ & $\textbf{29.5}$ \\
\bottomrule
\end{tabular}
% \begin{tablenotes}
% \item [*] They use different train / dev / test splits.
% \item [] 
% \end{tablenotes}
\end{threeparttable}
% \end{center}
% \caption{Evaluation results on VG VQA Japanese dataset.}
% \label{tab:jap_results}

% \end{table}
